# Supplementary material for: Designing Aqueous Organic Electrolytes for Zinc-Air Batteries: Method, Simulation, and Validation
Source: arXiv:1909.11461 ancillary file (2020-04-03)
Supplement: Supplementary file 1 [file supplementary_information.pdf]

# Supplementary Information - Designing Aqueous Organic Electrolytes for Zinc-Air Batteries: Method, Simulation, and Validation

Simon Clark,[1,2,3] Aroa R. Mainar,[4] Elena Iruin,[4] Luis C. Colmenares,[4] J. Alberto Blázquez,[4] Julian R. Tolchard,[3] Zenonas Jusys,[5] and Birger Horstmann[1,2,6,*]

[1]*German Aerospace Center, Pfaffenwaldring 38–40, 70569 Stuttgart, Germany*

[2]*Helmholtz Institute Ulm, Helmholtzstraße 11, 89081 Ulm, Germany*

[3]*SINTEF Industry, New Energy Solutions, Sem Saelands vei 12, 7034 Trondheim, Norway*

[4]*CIDETEC, Basque Research and Technology Alliance (BRTA), P° Miramón, 196, Donostia-San Sebastián 20014, Spain*

[5]*Institute of Surface Chemistry and Catalysis, Ulm University, Albert-Einstein-Allee 47, 89081 Ulm, Germany*

[6]*Faculty of Natural Sciences, Ulm University, 89081 Ulm, Germany*

* birger.horstmann@dlr.de

**CONTENTS**

S1. Theory, Model, and Parameterization S3
S1.1. Cell Reactions S3
S1.2. Thermodynamic Model S3
S1.3. Continuum Model S5
S1.4. Quasi-Particle Definitions S7
S1.4.1. Quasi-Particle Transport S8
S1.4.2. Reaction Kinetics S9
S1.5. Parameterization S10
S1.5.1. Thermodynamic Parameters S10
S1.5.2. Kinetic Parameters S14
S1.5.3. Transport Parameters S15

S2. Thermodynamic Screening of Electrolyte Materials S17

S3. Experimental Results S22
S3.1. Oxygen Electrocatalysis S22
S3.2. Full Cell Measurements S24
S3.3. Zn Electrode Characterisation S27

References S30

The supplementary information is divided into three parts. First, details of the modelling frameworks applied in this work are given in the section ***Theory, Model, and Parameterization***. Second, additional results and discussion on the electrolyte materials screening process are given in the section ***Thermodynamic Screening of Electrolyte Materials***. Third, additional experimental measurements of the electrolyte properties, full cell cycling performance, rotating ring disk electrode (RRDE) characterization, and XRD, SEM, and EDS measurements of the Zn electrode are presented in the section ***Experimental Results***.

## S1. THEORY, MODEL, AND PARAMETERIZATION

This study applies both thermodynamic models of chemical equilibrium and dynamic 1D continuum models to design new electrolyte materials and evaluate their performance in ZAB cells. Quasi-particle transport is derived in our previous works[1,2] and implemented in an existing framework for modelling metal-air batteries.[3–8] In this supplement, we provide an overview of the modelling method and parameterization.

### S1.1. Cell Reactions

The cell reactions laid out in Fig. 1 of the main text are listed here. For alkaline electrolytes:

$$\begin{aligned}
&\text{Ia:} && 0.5\,O_2 + H_2O + 2\,e^- \rightleftharpoons 2\,OH^- \\
&\text{IIa:} && Zn \rightleftharpoons Zn^{2+} + 2\,e^- \\
&\text{IIIa:} && Zn^{2+} + 4\,OH^- \rightleftharpoons Zn(OH)_4{}^{2-} \\
&\text{IVa:} && Zn(OH)_4{}^{2-} \rightleftharpoons ZnO + H_2O + 2\,OH^- \\
&\text{Va:} && CO_2 + 2\,OH^- \rightleftharpoons CO_3{}^{2-} + H_2O
\end{aligned}$$

For pH-buffered near-neutral electrolytes:

$$\begin{aligned}
&\text{Ib:} && 0.5\,O_2 + 2\,H^+ + 2\,e^- \rightleftharpoons H_2O \\
&\text{IIb:} && 2\,HA \rightleftharpoons 2\,H^+ + 2\,A^- \\
&\text{IIIb:} && Zn \rightleftharpoons Zn^{2+} + 2\,e^- \\
&\text{IVb:} && Zn^{2+} + xA^- \rightleftharpoons Zn(A)_x{}^{2-x} \\
&\text{Vb:} && Zn(A)_x{}^{2-x} + H_2O \rightleftharpoons ZnO + (x-2)\,A^- + 2HA
\end{aligned}$$

### S1.2. Thermodynamic Model

The thermodynamic speciation and solubility calculations presented in this work are based on the law of mass action,[9] which states that for a system in equilibrium, the reaction quotient of a given chemical reaction is a constant:

$$\prod a_i^{\nu_i} = \exp\left(\frac{-\sum \nu_i \mu_i^0}{RT}\right) = K_{\text{eq}}, \tag{1}$$

where $a_i$ is the activity of species $i$, $\nu_i$ is the stoichiometric coefficient of the species in the reaction, and $\mu_i^0$ is the standard chemical potential of the species. Here we assume an ideal

Table S1. Homogeneous electrolyte reactions in the mixed citric acid, glycine system.

| Reaction | $\log_{10} K_{eq}$ | Ref. |
|---|---|---|
| $H^+ + OH^- \rightleftharpoons H_2O$ | 13.96 | [10] |
| $H^+ + Cit^{3-} \rightleftharpoons HCit^{2-}$ | 5.33 | [11] |
| $H^+ + HCit^{2-} \rightleftharpoons H_2Cit^-$ | 4.08 | [11] |
| $H^+ + H_2Cit^- \rightleftharpoons H_3Cit$ | 2.87 | [11] |
| $H^+ + Gly^- \rightleftharpoons HGly$ | 9.63 | [11] |
| $H^+ + HGly \rightleftharpoons H_2Gly^+$ | 2.37 | [11] |
| $Zn^{2+} + HCit^{2-} \rightleftharpoons ZnHCit$ | 2.98 | [11] |
| $Zn^{2+} + Cit^{3-} \rightleftharpoons ZnCit^-$ | 4.27 | [11] |
| $Zn^{2+} + 2\,Cit^{3-} \rightleftharpoons {ZnCit_2}^{4-}$ | 5.90 | [11] |
| $Zn^{2+} + Gly^- \rightleftharpoons ZnGly^+$ | 4.90 | [11] |
| $Zn^{2+} + 2\,Gly^- \rightleftharpoons ZnGly_2$ | 8.98 | [11] |
| $Zn^{2+} + 3\,Gly^- \rightleftharpoons {ZnGly_3}^-$ | 11.29 | [11] |
| $Zn^{2+} + OH^- \rightleftharpoons Zn(OH)^+$ | 6.31 | [12] |
| $Zn^{2+} + 2\,OH^- \rightleftharpoons Zn(OH)_2$ | 11.19 | [12] |
| $Zn^{2+} + 3\,OH^- \rightleftharpoons {Zn(OH)_3}^-$ | 14.31 | [12] |
| $Zn^{2+} + 4\,OH^- \rightleftharpoons {Zn(OH)_4}^{2-}$ | 17.70 | [12] |

solution, $a = \gamma \frac{c_i}{c_0}$ with $\gamma = 1$. Similarly, the equilibrium potential of the electrochemical reactions are derived from expressions of thermodynamic equilibrium,[9] yielding the Nernst equation:

$$\phi_0 = \frac{\sum \nu_i \mu_i^0 + RT \sum \nu_i \ln a_i}{nF} = \phi_0^0 + \frac{RT}{nF} \sum \nu_i \ln(a_i) \tag{2}$$

Applying the law of mass action, the concentrations of the various complexes can be expressed in terms of their fundamental constituent components. For the proposed citric acid-glycine electrolyte, the homogeneous electrolyte reactions and their equilibrium stability constants are listed in Table S1.

Given that the pH of the electrolyte, total zinc concentration ($[Zn]_T$), total citrate concentration ($[Cit]_T$), and total glycine concentration ($[Gly]_T$) are known, the concentrations of the fundamental solutes $[H^+]$, $[OH^-]$, $[Cit^{3-}]$, $[Gly^-]$, $[K^+]$, and $[Zn^{2+}]$ can be calculated from the equations for mass and charge conservation.

$$[\mathrm{Zn}]_\mathrm{T} = [\mathrm{Zn}^{2+}] + \sum_{i=1}^{4} [\mathrm{Zn(OH)}_i^{\;2-i}] + [\mathrm{ZnHCit}] + \sum_{j=1}^{2} [\mathrm{Zn(Cit)}_j^{\;2-3j}] + \sum_{k=1}^{3} [\mathrm{Zn(Gly)}_k^{\;2-k}], \quad (3)$$

$$[\mathrm{Cit}]_\mathrm{T} = [\mathrm{Cit}^{3-}] + \sum_{l=1}^{3} [\mathrm{H}_l\mathrm{Cit}^{(3-l)}] + [\mathrm{ZnHCit}] + \sum_{j=1}^{2} j[\mathrm{Zn(Cit)}_j^{\;2-3j}], \quad (4)$$

$$[\mathrm{Gly}]_\mathrm{T} = [\mathrm{Gly}^{-}] + \sum_{m=1}^{2} [\mathrm{H}_m\mathrm{Gly}^{(1-m)}] + \sum_{k=1}^{3} k[\mathrm{Zn(Gly)}_k^{\;2-k}], \quad (5)$$

$$[\mathrm{OH}^-]_\mathrm{T} = [\mathrm{OH}^-] + \sum_{i=1}^{4} i[\mathrm{Zn(OH)}_\mathrm{i}^{\;2-\mathrm{i}}]. \quad (6)$$

$$[\mathrm{H}^+]_\mathrm{T} = [\mathrm{H}^+] + \sum_{l=1}^{3} [\mathrm{H}_l\mathrm{Cit}^{(3-l)}] + [\mathrm{ZnHCit}] + \sum_{m=1}^{2} [\mathrm{H}_m\mathrm{Gly}^{(1-m)}] \quad (7)$$

$$[\mathrm{K}^+] = \Big([\mathrm{OH}^-]_\mathrm{T} + [\mathrm{Gly}]_\mathrm{T} + 3[\mathrm{Cit}]_\mathrm{T}\Big) - \Big([\mathrm{H}^+]_\mathrm{T} + 2[\mathrm{Zn}]_\mathrm{T}\Big) \quad (8)$$

### S1.3. Continuum Model

The continuum model applied in this work is based on existing frameworks in the literature[3–5] and derived in detail in our existing works.[1,2] Here we give an overview of the relevant equations.

Quasi-particle continuum modelling is derived from concentrated solution theory of electrolyte transport[13] and the law of mass action[9] to efficiently model the dynamic behaviour of complex electrolytes. Assuming that homogeneous electrolyte reactions occur very quickly, *i.e.* infinitely fast, the system of continuity equations needed to describe electrolyte transport can be greatly simplified.

The quasi-particles must be defined to encompass the quantities of mass and charge that are conserved in the homogeneous electrolyte reactions. They are defined in terms of the weighted sum of the concentrations of their constituent components,

$$c_q = \sum_i \tau_{i,q} c_i, \quad (9)$$

where $\tau_{i,q}$ describes the stoichiometry of solute $i$ in quasi-particle $q$. The solute source term attributed to the homogeneous electrolyte speciation reactions is

$$\dot{s}_i^\mathrm{h} = \sum_r \tilde{k}_r^\mathrm{h} \nu_{i,r}. \quad (10)$$

In this equation, $\tilde{k}_r^{\mathrm{h}}$ is the rate of the homogeneous electrolyte reaction $r$ and $\nu_{i,r}$ is the stoichiometric coefficient of solute $i$ in the reaction. The source term of the quasi-particle due to the homogeneous electrolyte reactions is then expressed as

$$\dot{s}_q^{\mathrm{h}} = \sum_{i,r} \tilde{k}_r^{\mathrm{h}} \nu_{i,r} \tau_{i,q}. \tag{11}$$

Demanding that the definition of the quasi-particles upholds the relation $\sum_{i,r} \nu_{i,r}\tau_{i,q} = 0$, the quasi-particle source term, $\dot{s}_q^{\mathrm{h}} = 0$, vanishes for any reaction rates, $\tilde{k}_r^{\mathrm{h}}$. This approach allows the concentrations of the many solutes to be easily determined from the concentrations of just a few quasi-particles.

In our previous works, we have derived quasi-particle models to simulate the dynamic behavior of $NH_4Cl-ZnCl_2$ electrolytes. Here we show how the framework can be adapted to a more general form for modelling a variety of electrolyte compositions.

First, consider a simple aqueous electrolyte system comprising $KOH-ZnO-H_2O$. The electrolyte contains the elementary species $K^+$, $OH^-$, $H^+$, $Zn^{2+}$, and the zinc complexes $Zn(OH)^+$, $Zn(OH)_2$, ${Zn(OH)_3}^-$, and ${Zn(OH)_4}^{2-}$. In this system, there are a total of 8 solutes ($n_{\mathrm{s}}$) and 5 homogeneous reaction equations ($n_{\mathrm{hr}}$). The number of quasi-particles ($n_{\mathrm{q}}$) required to describe the system is $n_{\mathrm{q}} = n_{\mathrm{s}} - n_{\mathrm{hr}} - 1 = 2$. The state of the system is determined by the concentration of $Zn^{2+}$ and the pH. $\widetilde{\mathrm{Zn}}$ is defined as the sum of all $Zn^{2+}$ (both free and complexed) and $\widetilde{\mathrm{HOH}}$ is the sum of all $H^+$ less the sum of all $OH^-$ in the solution,

$$[\widetilde{\mathrm{Zn}}] = [\mathrm{Zn}^{2+}] + \sum_{i=1}^{4} [{\mathrm{Zn(OH)}_i}^{2-i}], \tag{12}$$

$$[\widetilde{\mathrm{HOH}}] = [\mathrm{H}^+] - \left( [\mathrm{OH}^-] + \sum_{i=1}^{4} i[{\mathrm{Zn(OH)}_i}^{2-i}] \right). \tag{13}$$

This is the simplest form of the quasi-particle description of aqueous zinc electrolytes, and it is sufficient to describe standard alkaline ZABs. These definitions provide a foundation that can be expanded to model more complex systems.

We now add some generic weak acid HA, and an additional quasi-particle, $\widetilde{\mathrm{A}}$, is needed. With this extra component, the quasi-particle definitions become

$$[\widetilde{\mathrm{Zn}}] = [\mathrm{Zn}^{2+}] + \sum_{i=1}^{4} [{\mathrm{Zn(OH)}_i}^{2-i}] + \sum_j [{\mathrm{Zn(A)}_j}^{2-j}] + \sum_k \sum_l [\mathrm{Zn(OH)}_k{(\mathrm{A})_l}^{2-(k+l)}], \tag{14}$$

$$[\widetilde{\mathrm{A}}] = [\mathrm{A}^-] + [\mathrm{HA}] + \sum_j j[{\mathrm{Zn(A)}_j}^{2-j}] + \sum_k \sum_l l[\mathrm{Zn(OH)}_k{(\mathrm{A})_l}^{2-(k+l)}], \tag{15}$$

$$[\widetilde{\mathrm{HOH}}] = \Big([\mathrm{H^+}] + [\mathrm{HA}]\Big) - \Big([\mathrm{OH^-}] + \sum_{i=1}^{4} i[\mathrm{Zn(OH)}_i{}^{2-i}] + \sum_k \sum_l k[\mathrm{Zn(OH)}_k(\mathrm{A})_l{}^{2-(k+l)}]\Big). \quad (16)$$

These generic definitions assume a monoprotic weak acid with a negatively-charged conjugate base; they can be easily modified to accommodate weak acids with other properties. Further components can be added to the electrolyte through the inclusion of additional quasi-particles.

With this model, we simulate the performance of a lab-scale cell with aqueous organic electrolytes. The resulting simulations give an idea of the feasibility of the system, help to interpret experimental results, and guide the future development of the system. All simulations presented in this study are performed using MATLAB R2018b.

### S1.4. Quasi-Particle Definitions

As discussed in the main text, the definition of the quasi-particles must be made to reflect the quantities of mass and charge conserved in the electrolyte, such that $\sum_{i,r} \nu_{i,r}\tau_{i,q} = 0$. The quasi-particles are $\widetilde{\mathrm{Zn}}$, $\widetilde{\mathrm{Cit}}$, $\widetilde{\mathrm{Gly}}$, and $\widetilde{\mathrm{HOH}}$, and they are defined as:

$$[\widetilde{\mathrm{Zn}}] = [\mathrm{Zn^{2+}}] + \sum_{i=1}^{4} [\mathrm{Zn(OH)}_i{}^{2-i}] + [\mathrm{ZnHCit}] + \sum_{j=1}^{2} [\mathrm{Zn(Cit)}_j{}^{2-3j}] + \sum_{k=1}^{3} [\mathrm{Zn(Gly)}_k{}^{2-k}], \quad (17)$$

$$[\widetilde{\mathrm{Cit}}] = [\mathrm{Cit^{3-}}] + \sum_{l=1}^{3} [\mathrm{H}_l\mathrm{Cit}^{(3-l)}] + [\mathrm{ZnHCit}] + \sum_{j=1}^{2} j[\mathrm{Zn(Cit)}_j{}^{2-3j}], \quad (18)$$

$$[\widetilde{\mathrm{Gly}}] = [\mathrm{Gly^-}] + \sum_{m=1}^{2} [\mathrm{H}_m\mathrm{Gly}^{(1-m)}] + \sum_{k=1}^{3} k[\mathrm{Zn(Gly)}_k{}^{2-k}], \quad (19)$$

$$[\widetilde{\mathrm{HOH}}] = \Big([\mathrm{H^+}] + \sum_{l=1}^{3} [\mathrm{H}_l\mathrm{Cit}^{(3-l)}] + [\mathrm{ZnHCit}] + \sum_{m=1}^{2} [\mathrm{H}_m\mathrm{Gly}^{(1-m)}]\Big) - \Big([\mathrm{OH^-}] + \sum_{i=1}^{4} i[\mathrm{Zn(OH)}_\mathrm{i}{}^{2-\mathrm{i}}]\Big). \quad (20)$$

The conservations of mass and charge in this system are:

$$[\mathrm{Zn}]_\mathrm{T} = [\widetilde{\mathrm{Zn}}] \quad (21)$$

$$[\mathrm{Cit}]_\mathrm{T} = [\widetilde{\mathrm{Cit}}] \quad (22)$$

$$[\mathrm{Gly}]_\mathrm{T} = [\widetilde{\mathrm{Gly}}] \quad (23)$$

$$[\mathrm{K}]_\mathrm{T} = 2[\widetilde{\mathrm{Zn}}] - 3[\widetilde{\mathrm{Cit}}] - [\widetilde{\mathrm{Gly}}] + [\widetilde{\mathrm{HOH}}]. \quad (24)$$

*S1.4.1. Quasi-Particle Transport*

The continuity equations for quasi-particle, $q$, mass and charge in the electrolyte are:

$$\frac{\partial(c_q \varepsilon_e)}{\partial t} = \underbrace{-\vec{\nabla} \cdot \vec{N}_q^{\mathrm{D,M}} - \vec{\nabla} \cdot \vec{N}_q^{\mathrm{C}}}_{\text{transport}} + \overbrace{\dot{s}_i}^{\text{source}}, \quad (25)$$

$$0 = \underbrace{-\vec{\nabla} \cdot \vec{j}}_{\text{transport}} + \overbrace{\sum_q z_q \dot{s}_q}^{\text{source}}. \quad (26)$$

Solving the continuity equations at each time step yields concentrations for the quasi-particles, $c_q$. Assuming that the homogeneous reactions occur very quickly, the law of mass action is applied to calculate the concentrations of each constituent solute, $c_i$. The diffusion-migration flux of the quasi-particles, $\vec{N}_q^{\mathrm{D,M}}$, is calculated as the weighted sum of diffusion-migration flux of its constituent components:

$$\vec{N}_q^{\mathrm{D,M}} = \varepsilon_\mathrm{e}^\beta \sum_i \tau_{i,q} D_i \vec{\nabla} c_i + \sum_i \tau_{i,q} \frac{t_i}{z_i F} \vec{j} \quad (27)$$

The electrolyte current density, $\vec{j}$, is:

$$\vec{j} = -\kappa \vec{\nabla} \phi_e + \frac{\kappa}{F} \sum_{i=1}^{h} \frac{t_i}{z_i} \frac{\partial \mu_i}{\partial c_i} \vec{\nabla} c_i. \quad (28)$$

The convective flux can be expressed in terms of the center-of-mass velocity of the electrolyte

$$\vec{N}_q^{\,\mathrm{C}} = c_q \vec{v}_e. \quad (29)$$

The electrolyte velocity is driven by the pressure gradient in the electrolyte, as stated in Darcy's Law:

$$\vec{v}_e = -\frac{B_e}{\eta_e} \vec{\nabla} p_e, \quad (30)$$

where $\eta_e$ is the viscosity of the electrolyte. The pressure is determined such that the electrolyte equation of state (derived from the Gibbs-Duhem relation) remains fulfilled,

$$\sum \bar{V}_i c_i = 1, \quad (31)$$

In porous media, the difference of electrolyte pressure ($p_\mathrm{c}$) and gas pressure ($p_\mathrm{cap}$) is defined as the capillary pressure ($p_\mathrm{c}$). The capillary pressure is linked to the electrolyte saturation in the porous structure using a Leverett approach,

$$J(s) = \sqrt{\frac{B_e}{\varepsilon_0 \sigma^2}} p_\mathrm{cap} = A + Be^{C(s-0.5)} - De^{-E(s-0.5)}. \tag{32}$$

The fitting parameters $A...E$ are listed in Table S8.

Finally, we add an additional transport equation to describe the mass continuity of the bulk electrolyte,

$$\frac{\partial(\rho \varepsilon_\mathrm{e})}{\partial t} = \vec{\nabla} \cdot \left(\varepsilon_\mathrm{e}^{\beta} \rho \vec{v_\mathrm{e}}\right) + \sum_q M_q \dot{s}_q. \tag{33}$$

*S1.4.2. Reaction Kinetics*

The electrochemical charge-transfer reactions are modelled with the Butler-Volmer approximation,[14]

$$k = k_0 \left( \exp\left[ \frac{\alpha RT}{nF} \eta \right] - \exp\left[ - \frac{(1-\alpha)RT}{nF} \eta \right] \right), \tag{34}$$

where $k_0$ is the reaction rate constant (linked to the exchange current density), $\alpha$ is the symmetry factor, $\eta$ is the surface overpotential, and the other variables take on their usual meaning.[15] The specific surface area for the reaction is consant in the cathode and a function of Zn volume fraction in the anode:

$$A^\mathrm{sp}_\mathrm{anode} = \frac{6}{a_\mathrm{s}} \varepsilon_\mathrm{Zn} (1 - \varepsilon_\mathrm{Zn}), \tag{35}$$

where $a_\mathrm{s}$ is the pore size of the Zn electrode and $\varepsilon_\mathrm{Zn}$ is the Zn metal solid volume fraction.

Precipitation reactions occur when the concentration of aqueous zinc species exceeds the solubility limit. The rate of these reactions is assumed to be diffusion limited. It is described by the diffusion of the limiting species and the degree to which the solubility has been exceeded:

$$k_r = \frac{D_\mathrm{Zn}}{\delta} \frac{\left(c_\mathrm{Zn} - c_r^\mathrm{sat}\right)}{c^0_\mathrm{Zn}}, \tag{36}$$

where $D_\mathrm{Zn}$ is the zinc diffusion coefficient, $\delta$ is the diffusion length, $c_\mathrm{Zn}$ is the aqueous zinc concentration, and $c_r^\mathrm{sat}$ is the zinc saturation concentration of the solid. We define the specific surface area for the precipitation reactions as:

$$A^\mathrm{sp}_p = \frac{6}{a_\mathrm{s}} \varepsilon_\mathrm{s} (1 - \varepsilon_\mathrm{s}), \tag{37}$$

where $a_\mathrm{s}$ is the pore size of the solid phase and $\varepsilon_\mathrm{s}$ is the total solid volume fraction.

The dissolution of oxygen into the electrolyte from the gas phase is modeled as described in existing works.[3,4] The solubility of oxygen in the electrolyte is determined by Henry's law, $[{O_2}^\mathrm{aq}] = H p_{O_2}$. The kinetics of the reaction are defined as $k_{O_2} = k_s^\mathrm{f} p_{O_2} - k_s^\mathrm{b} [O_2]$.

Table S2. Reactions that contribute to the quasi-particle source terms.

| Reaction | In Terms of Quasi-Particles |
| --- | --- |
| $0.5\,O_2 + 2\,H^+ + 2\,e^- \rightleftharpoons H_2O$ | $0.5\,O_2 + 2\,\widetilde{HOH} + 2\,e^- \rightleftharpoons H_2O$ |
| $Zn(s) \rightleftharpoons Zn^{2+} + 2\,e^-$ | $Zn(s) \rightleftharpoons \widetilde{Zn} + 2\,e^-$ |
| $Zn^{2+} + H_2O \rightleftharpoons ZnO(s) + 2\,H^+$ | $\widetilde{Zn} + H_2O \rightleftharpoons ZnO(s) + 2\,\widetilde{HOH}$ |
| $Zn^{2+} + 2\,H_2O \rightleftharpoons Zn(OH)_2(s) + 2\,H^+$ | $\widetilde{Zn} + 2\,H_2O \rightleftharpoons Zn(OH)_2(s) + 2\,\widetilde{HOH}$ |
| $3\,Zn^{2+} + 2\,Cit^{3-} \rightleftharpoons Zn_3Cit_2(s)$ | $3\,\widetilde{Zn} + 2\,\widetilde{Cit} \rightleftharpoons Zn_3Cit_2(s)$ |

The various reactions, $r$, contribute to the quasi-particle source terms as:

$$\dot{s}_q = \sum_i \sum_r \tau_{i,q} \nu_{i.r} k_r A_r^{\mathrm{sp}}. \tag{38}$$

A list of reactions that contribute to the quasi-particle source terms is given in Table S2.

### S1.5. Parameterization

This section provides a list of parameters for the implementation of the models described above.

#### *S1.5.1. Thermodynamic Parameters*

Homogeneous electrolyte reactions and their stability constants for selected alternative counterions and pH buffers are listed in Tables S3 and S4, respectively. Solubility product constants for some sparingly soluble zinc salts of interest are listed in Table S5. The solubility product constants of the listed salts are normalized to describe a stoichiometry of Zn = 1.

Table S3. Homogeneous electrolyte reactions for some alternative inorganic counterions considered in this work.

| Reaction | $\log_{10} K_{eq}$ | Ref. |
|---|---|---|
| **Counterions** | | |
| $Zn^{2+} + SO_4{}^{2-} \rightleftharpoons ZnSO_4$ | 0.70 | [10] |
| $Zn^{2+} + 2\,SO_4{}^{2-} \rightleftharpoons Zn(SO_4)_2{}^{2-}$ | 0.70 | [10] |
| $Zn^{2+} + 3\,SO_4{}^{2-} \rightleftharpoons Zn(SO_4)_3{}^{4-}$ | 0.90 | [10] |
| $Zn^{2+} + 4\,SO_4{}^{2-} \rightleftharpoons Zn(SO_4)_4{}^{6-}$ | 0.90 | [10] |
| $Zn^{2+} + NO_3{}^{-} \rightleftharpoons ZnNO_3{}^{+}$ | 0.01 | [10] |
| $Zn^{2+} + 2\,NO_3{}^{-} \rightleftharpoons Zn(NO_3)_2$ | -1.10 | [10] |

Table S4. Homogeneous electrolyte reactions for some alternative pH buffers considered in this work.

| Reaction | $\log_{10} K_{\mathrm{eq}}$ | Ref. |
|---|---|---|
| **pH Buffers** | | |
| $NH_3 + H^+ \rightleftharpoons NH_4^+$ | 9.8 | [10] |
| $Zn^{2+} + NH_3 \rightleftharpoons ZnNH_3^{2+}$ | 2.38 | [10] |
| $Zn^{2+} + 2\,NH_3 \rightleftharpoons Zn(NH_3)_2^{2+}$ | 4.88 | [10] |
| $Zn^{2+} + 3\,NH_3 \rightleftharpoons Zn(NH_3)_3^{2+}$ | 7.43 | [10] |
| $Zn^{2+} + 4\,NH_3 \rightleftharpoons Zn(NH_3)_4^{2+}$ | 9.65 | [10] |
| $PO_4^{3-} + H^+ \rightleftharpoons HPO_4^{2-}$ | 10.79 | [10] |
| $HPO_4^{2-} + H^+ \rightleftharpoons H_2PO_4^-$ | 6.26 | [10] |
| $H_2PO_4^- + H^+ \rightleftharpoons H_3PO_4$ | 1.86 | [10] |
| $Zn^{2+} + HPO_4^{2-} \rightleftharpoons ZnHPO_4$ | 2.4 | [10] |
| $Zn^{2+} + H_2PO_4^- \rightleftharpoons ZnH_2PO_4^+$ | 1.2 | [10] |
| $CO_3^{2-} + H^+ \rightleftharpoons HCO_3^-$ | 9.56 | [10] |
| $HCO_3^- + H^+ \rightleftharpoons H_2CO_3$ | 6.33 | [10] |
| $Zn^{2+} + HCO_3^- \rightleftharpoons ZnHCO_3^+$ | 2.1 | [16] |
| $Zn^{2+} + CO_3^{2-} \rightleftharpoons ZnCO_3$ | 5.3 | [16] |
| $CN^- + H^+ \rightleftharpoons HCN$ | 9.48 | [10] |
| $Zn^{2+} + CN^- \rightleftharpoons ZnCN^+$ | 5.3 | [10] |
| $Zn^{2+} + 2\,CN^- \rightleftharpoons Zn(CN)_2$ | 11.7 | [10] |
| $Zn^{2+} + 3\,CN^- \rightleftharpoons Zn(CN)_3^-$ | 16.7 | [10] |
| $Zn^{2+} + 4\,CN^- \rightleftharpoons Zn(CN)_4^{2-}$ | 21.6 | [10] |
| $Im + H^+ \rightleftharpoons HIm^+$ | 7.31 | [17] |
| $Zn^{2+} + Im \rightleftharpoons ZnIm^{2+}$ | 2.56 | [17] |
| $Zn^{2+} + 2\,Im \rightleftharpoons Zn(Im)_2^{2+}$ | 4.89 | [17] |
| $Zn^{2+} + 3\,Im \rightleftharpoons Zn(Im)_3^{2+}$ | 7.16 | [17] |
| $Zn^{2+} + 4\,Im \rightleftharpoons Zn(Im)_4^{2+}$ | 9.19 | [17] |

Table S5. Solubility product constants, normalized to stoichiometry Zn = 1.

| Reaction | $\log_{10} K_{sp}$ | Ref. |
|---|---|---|
| $Zn(OH)_2 \rightleftharpoons Zn^{2+} + 2\,OH^-$ | -16.52 | [18] |
| $ZnO \rightleftharpoons Zn^{2+} + 2\,OH^-$ | -16.85 | [18] |
| $Zn(OH)_{1.6}Cl_{0.4} \cdot H_2O \rightleftharpoons Zn^{2+} + 1.6\,Cl^- + 0.4\,OH^- + H_2O$ | -14.2 | [18] |
| $Zn(PO_4)_{2/3} \cdot 4\,H_2O \rightleftharpoons Zn^{2+} + \frac{2}{3}\,PO_4{}^{3-}$ | -11.76 | [10] |
| $Zn(OH)_{1.5}(SO_4)_{0.2} \cdot 4\,H_2O \rightleftharpoons Zn^{2+} + 0.2\,SO_4{}^{2-} + 1.5\,OH^-$ | -13.9 | [18] |
| $Zn(OH)_{1.75}(ClO_4)_{0.25} \rightleftharpoons Zn^{2+} + 0.25\,ClO_4{}^- + 1.75\,OH^-$ | -15.19 | [18] |
| $Zn(OH)_{1.6}(NO_3)_{0.4} \rightleftharpoons Zn^{2+} + 0.4\,NO_3{}^- + 1.6\,OH^-$ | -10.13 | [19] |
| $ZnCO_3 \rightleftharpoons Zn^{2+} + CO_3{}^{2-}$ | -10 | [10] |
| $Zn(OH)_{1.6}(CO_3)_{0.4} \rightleftharpoons Zn^{2+} + 0.4\,CO_3{}^- + 1.6\,OH^-$ | -14.7 | [18] |
| $Zn(Cit)_{2/3} \rightleftharpoons Zn^{2+} + \frac{2}{3}\,Cit^{3-}$ | -3.66 | [20] |

*S1.5.2. Kinetic Parameters*

Kinetic parameters implemented in the quasi-particle continuum model are listed in Table S6.

Table S6. Kinetic parameters for the electrochemical reactions.[21]

| Parameter | Value | Unit |
|---|---|---|
| $k_0^{\mathrm{Zn}}$ | $10^{-5.1}$ | $\mathrm{mol \cdot m^{-2} \cdot s^{-1}}$ |
| $\alpha_a^{\mathrm{Zn}}$ | 0.5 | - |
| $\alpha_c^{\mathrm{Zn}}$ | 0.5 | - |
| $A_{\mathrm{sp}}^{\mathrm{Zn}}$ | $f(\varepsilon_{\mathrm{Zn}})$ | $\mathrm{m^{-2} \cdot m^{-3}}$ |
| $a_0$ | $100 \times 10^{-6}$ | m |
| $k_0^{\mathrm{GDE}}$ | $10^{-8.4}$ | $\mathrm{mol \cdot m^{-2} \cdot s^{-1}}$ |
| $\alpha_a^{\mathrm{GDE}}$ | 0.5 | - |
| $\alpha_c^{\mathrm{GDE}}$ | 0.5 | - |
| $A_{\mathrm{sp}}^{\mathrm{GDE}}$ | $4.5 \times 10^3$ | $\mathrm{m^{-2} \cdot m^{-3}}$ |

### *S1.5.3. Transport Parameters*

A list of the transport parameters implemented in the model is given in Table S7. Transport parameters for citric acid species are compiled by Apelblat.[22] Transport parameters for glycine are estimated according to those reported by Hamborg et al.[23] Other transport parameters have yet to be investigated in existing experimental studies. Parameter estimates here are chosen to reflect the order-of-magnitude. Detailed experimental determination of these transport parameters could be a topic for further research.

Table S7. Estimated transport parameters of aqueous citrate and glycine species.

| Species | $M_i$ / $g \cdot mol^{-1}$ | $z_i$ / – | $D_i \times 10^9$ / $m^2 \cdot s^{-1}$ | $\lambda_i^0 \times 10^4$ / $S \cdot m^2 \cdot equiv^{-1}$ | $\bar{V}_i \times 10^6$ / $m^3 \cdot mol^{-1}$ |
|---|---|---|---|---|---|
| $H_3Cit$ | 192.1 | 0 | 0.66 | 0 | 100 |
| $H_2Cit^-$ | 191.1 | -1 | 0.81 | 35.87 | 100 |
| $HCit^{2-}$ | 190.1 | -2 | 0.81 | 50.38 | 100 |
| $Cit^{3-}$ | 189.1 | -3 | 0.76 | 72.05 | 100 |
| $H_2Gly^+$ | 76.1 | +1 | 1.11 | 30 | 20 |
| HGly | 75.1 | 0 | 1.11 | 0 | 20 |
| $Gly^-$ | 74.1 | -1 | 1.11 | 30 | 20 |
| ZnHCit | 254.5 | 0 | 0.2 | 0 | 100 |
| $ZnCit^-$ | 253.5 | -1 | 0.2 | 50 | 100 |
| ${ZnCit_2}^{4-}$ | 442.6 | -4 | 0.2 | 80 | 150 |
| $ZnGly^+$ | 139.4 | +1 | 0.5 | 30 | 10 |
| $ZnGly_2$ | 213.5 | 0 | 0.5 | 0 | 20 |
| ${ZnGly_3}^-$ | 287.6 | -1 | 0.5 | 30 | 40 |

Table S8. Leverett function parameters.

| Coefficient | Value |
|---|---|
| A | 0.1872 |
| B | 0.02523 |
| C | 8.707 |
| D | 0.09515 |
| E | 5.622 |

## S2. THERMODYNAMIC SCREENING OF ELECTROLYTE MATERIALS

Figure S1 lays out the design criteria established in this work for aqueous electrolytes for Zn-air batteries. An ideal aqueous electrolyte should meet some fundamental requirements to promote good ZAB operation (Fig. S1†). (i) The pH of the electrolyte should be relatively stable during operation. Large swings in operational pH can degrade battery materials (especially in the air electrode) and reduce lifetime. A functionally stable pH can be achieved through the use of concentrated alkaline/acidic electrolytes or the incorporation of a pH-buffer .[2] (ii) $Zn^{2+}$ should be moderately soluble in the solution. The goal is to allow $Zn^{2+}$ to escape the surface of the Zn electrode and avoid passivation, but not diffuse so far away as to contribute to Zn electrode shape change. When precipitated discharge products form, they should be dominated by a porous ZnO phase.[1] (iii) The kinetics of the ORR/OER are the major limitations to ZAB efficiency and rate-capability.[24,25] The electrolyte should not inhibit these reactions, *e.g.* by blocking active catalyst sites. (iv) To facilitate mass transport within the ZAB cell, the electrolyte should be highly ionically conductive and non-viscous. (v) Because ZABs are semi-open systems, some leakage of the electrolyte cannot be ruled out. Therefore, toxic or environmentally harmful materials should be avoided. (vi) For the battery to have a long lifetime, the electrolyte should be stable in air and within the electrochemical window of the cell.[3,26] Furthermore, (vii) the vapor pressure of the electrolyte should be low to avoid evaporation losses out of the air electrode. An electrolyte with such properties could be a good candidate for rechargeable ZAB applications.

As part of the material screening process, we identify the dissociation constants of weak acids and the equilibrium stability constants of their conjugate bases with $Zn^{2+}$ as thermodynamic descriptors. These values give insight into $Zn^{2+}$ solubility, ZnO favorability, and pH buffering capacity.

$Zn(SO_4)$ electrolytes have recently attracted significant attention for use in Zn-ion batteries.[27–30] Sulfate anions, ${SO_4}^{2-}$, form weak complexes with $Zn^{2+}$, but $Zn_4(OH)_6SO_4$ is only sparingly soluble for near-neutral pH values.[31] Electrolytes containing nitrate anions,[32,33] ${NO_3}^-$, can precipitate $Zn(OH)_8(NO_3)_2$. ${NO_3}^-$ ions are also strong oxidants and are subject to a redox shuttle, as is known from Ni-Cd and Ni-MH batteries.[34,35] Similar solubility challenges afflict perchlorate, ${ClO_4}^-$, and phosphate, ${PO_4}^{3-}$, counter-ions.[18] Tetrafluoroborate, ${BF_4}^-$, and hexafluorophosphate, ${PF_6}^-$, are common anions in ionic liquid electrolytes, but they undergo hydrolysis reactions in aqueous solutions[36,37] with the potential to form toxic and environmentally harmful degradation products like HF. Finally, recent research has shown the promise of bulky anions like triflate, $CF_3{SO_3}^-$,[38,39] and bistriflimide (TFSI), $(CF_3SO_2)_2N^-$,[40] to reduce parasitic $H_2$ evolution and improve Zn metal deposition. However, these materials are currently far too expensive to support the low cost targets of ZABs.

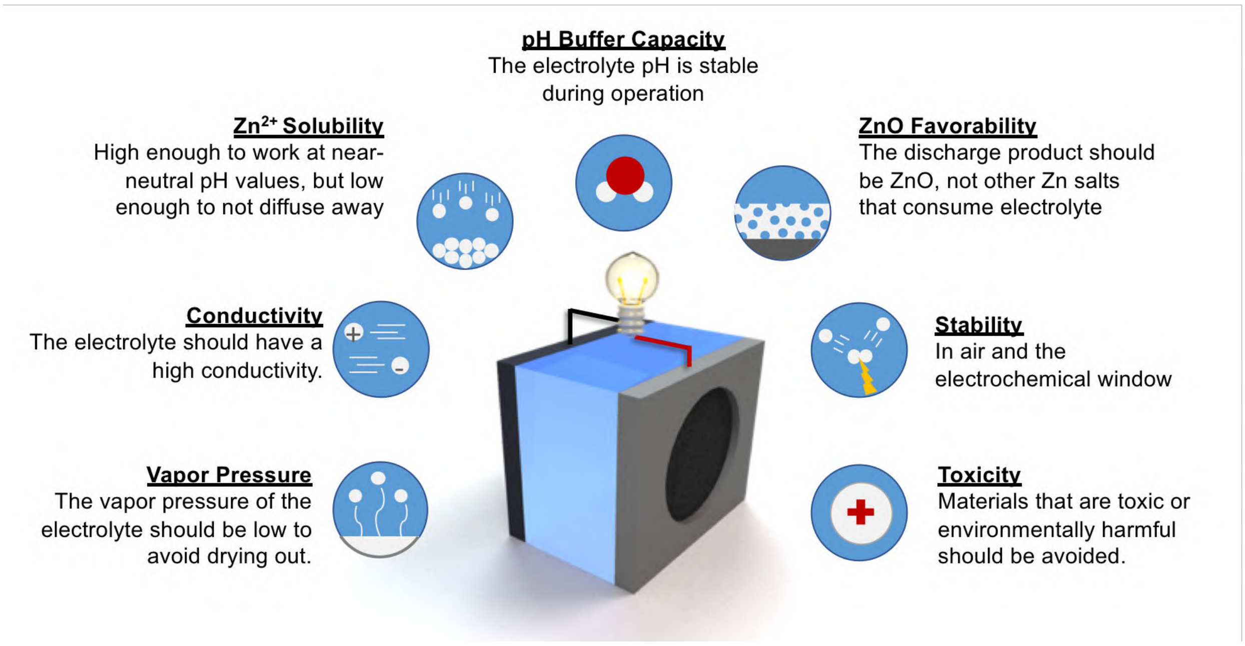


Figure S1. Overview of factors to consider in aqueous Zn electrolyte design.

Inorganic pH-buffers like $H_3PO_4$, $H_2CO_3$, or HCN could potentially address some of these challenges. In these examples, the acid is charge-neutral and the conjugate base is negatively charged, avoiding the need for a negative counter-ion. Furthermore, because of their polyprotic nature (except HCN), these acids can buffer pH at multiple levels, improving the resilience of the battery against unstable pH shifts. But the solubilities of mixed zinc phosphates and carbonates are still very low and threaten the precipitation of ZnO as the dominant discharge product.[10,18] Additionally, cyanide is highly toxic and unsuitable for a semi-open system. These materials do not offer an outstanding alternative to ${NH_4}^+$. Thermodynamic speciation and solubility landscapes for some alternative counter-ions and pH buffers are given in Figs. S2 and S3†.

Alternative negative counterions like ${SO_4}^{2-}$, ${NO_3}^-$, and ${ClO_4}^-$ are challenging due to both their strongly oxidizing nature and the tendency to form insoluble zinc salts at near-neutral pH values. Unwanted precipitation of zinc salts also afflicts alternative pH buffers like $H_3PO_4$, $H_2CO_3$, and HCN. Solubility product constants of selected zinc salts are listed in Table S5, and alternative speciation and solubility landscapes are shown in Figure S2.

Carboxylic acids (*e.g.* citric acid) and aminocarboxylic acids (*e.g.* glycine) have been cited as components in electrolytes for both battery and electroplating applications.[41–57] However, one of the challenges facing these materials in aqueous electrolytes relates to their electrochemical stability. The electro-oxidation of glycinate on Pt surfaces was investigated by Marangoni, et al. in 1989.[58] They proposed that in a basic solution, the oxidation of

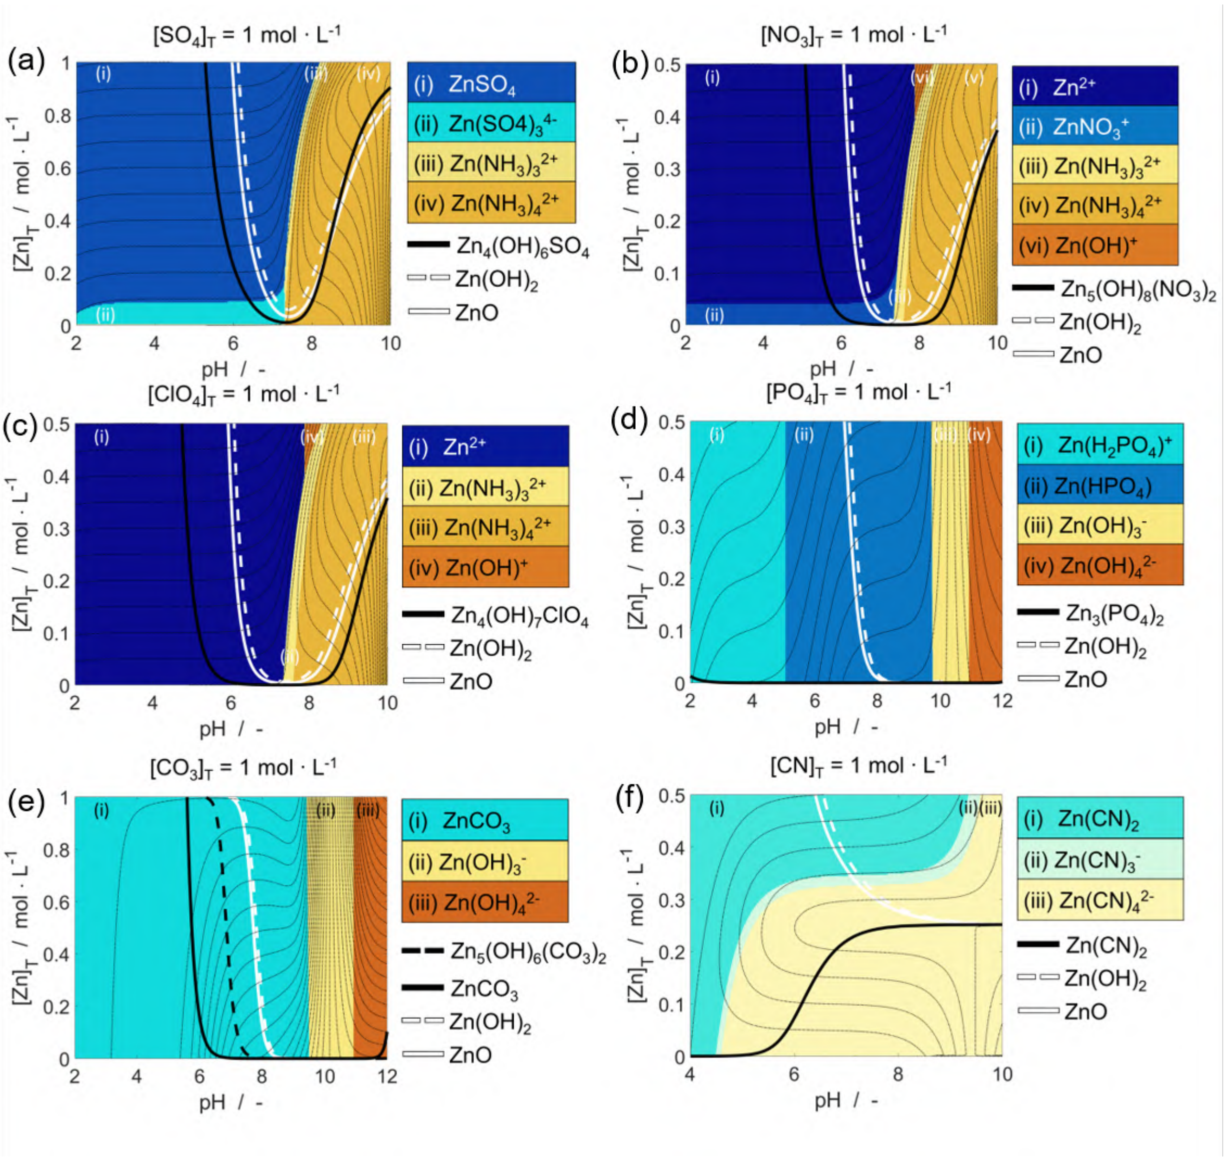


Figure S2. Speciation and solubility landscapes of some alternative inorganic electrolyte materials. Colored regions indicate the dominant zinc complex in the electrolyte, Thick white and black lines indicate the solubility limits of various solid products, and thin dotted lines indicate iso-paths tracing electrolyte composition shifts as the cell is discharged ($[Zn]_T$ increases) and charged ($[Zn]_T$ decreases). For alternative conunterion systms - (a) $SO_4{}^{2-}$, (b) $NO_3{}^{-}$, and (c) $ClO_4{}^{-}$ - the pH buffering species is $NH_4{}^{+}$. For alternative pH buffers - (d) $H_3PO_4$, (e) $H_2CO_3$, and (f) HCN - the counterion is $K^+$.

glycinate occurs via the overall reaction:

$$C_2H_4NO_2{}^- + OH^- \longrightarrow CH_2O + NH_3 + CO_2 + 2\,e^-. \tag{39}$$

More recently, the oxidation of glycine in an acidic solution was proposed by Hamelers, et

al.[59] to occur via the reaction:

$$C_2H_5NO_2 + 4\,H_2O \longrightarrow 2\,HCO_3{}^- + 7\,H^+ + NH_4{}^+ + 6\,e^-. \tag{40}$$

Likewise, the complete oxidation of citrate in a basic solution occurs via the overall reaction:

$$C_6H_5O_7{}^{3-} + 27\,OH^- \longrightarrow 6\,CO_3{}^{2-} + 16\,H_2O + 18\,e^-. \tag{41}$$

Considering the standard Gibbs free energies of formation for the various components, the standard redox potentials for complete glycine and citrate oxidation are -0.97 V and -0.89 V, respectively. The standard potential of the air electrode in a basic solution is 0.401 V. The thermodynamics of the system favor some decomposition of these species in the electrolyte during cell operation. However, the redox properties of organic molecules are complex and they can form myriad reaction intermediates before being completely oxidized to $CO_3{}^{2-}$ or $CO_2$. The RRDE analysis presented in this work indicates that, while oxidation of the organic electrolyte components during cell charging is a problem, proper catalyst selection can yield improved OER activity.

One interesting alternative to carboxylic and aminocarboxylic acids are the azoles, namely imidazole. Imidazole acts as an effective $Zn^{2+}$ chelator and can accept a proton to become imidazolium, buffering pH around 7.58. However, imidazolium requires a negatively charged counterion. Additionally, the cost of imidazole is significantly higher than citric acid and glycine. Nonetheless, we present here the thermodynamic dissociation and speciation diagrams for aqueous mixtures of imidazolium and zinc.

Imidazolium cations are currently widely researched for ionic liquid electrolytes, but they could also be of interest in aqueous electrolyte development.[42,60] Imidazolium has a proton in the N-3 location with a $pK_a$ value of 7.31.[17] The imidazolium ring can be modified to include a variety of functional groups. For example 4-(2-Aminoethyl)imidazolium is able to donate a second proton from the amine group with a $pK_a$ value of 9.88.[17] Ionic liquid electrolytes often include 1-ethyl-3-methylimidazolium, but as the N-3 position is occupied by a methyl group, the $pK_a$ is outside the range that would be appropriate for aqueous ZAB pH buffering.[61]

Figure S3 shows (a) the dissociation and (b) $Zn^{2+}$ speciation properties of imidazolium solutions. In aqueous solution, imidazolium can donate a single proton ($pK_a = 7.31$) and become the charge-neutral species imidazole. When zinc ions are introduced to the system, the speciation is dominated by $Zn^{2+}$ for acidic pH values, $Zn(Im)_4{}^{2+}$ between pH 5-12, and $Zn(OH)_4{}^{2-}$ for alkaline pH values.

From the thermodynamic analysis, we can make a few statements regarding the practical uses of these materials for aqueous ZAB electrolyte applications. Imidazolium shows suitable pH buffering and $Zn^{2+}$ complexing properties, but the $pK_a$ value is slightly too low to adequately stabilize the pH during cell operation. Furthermore, because it can

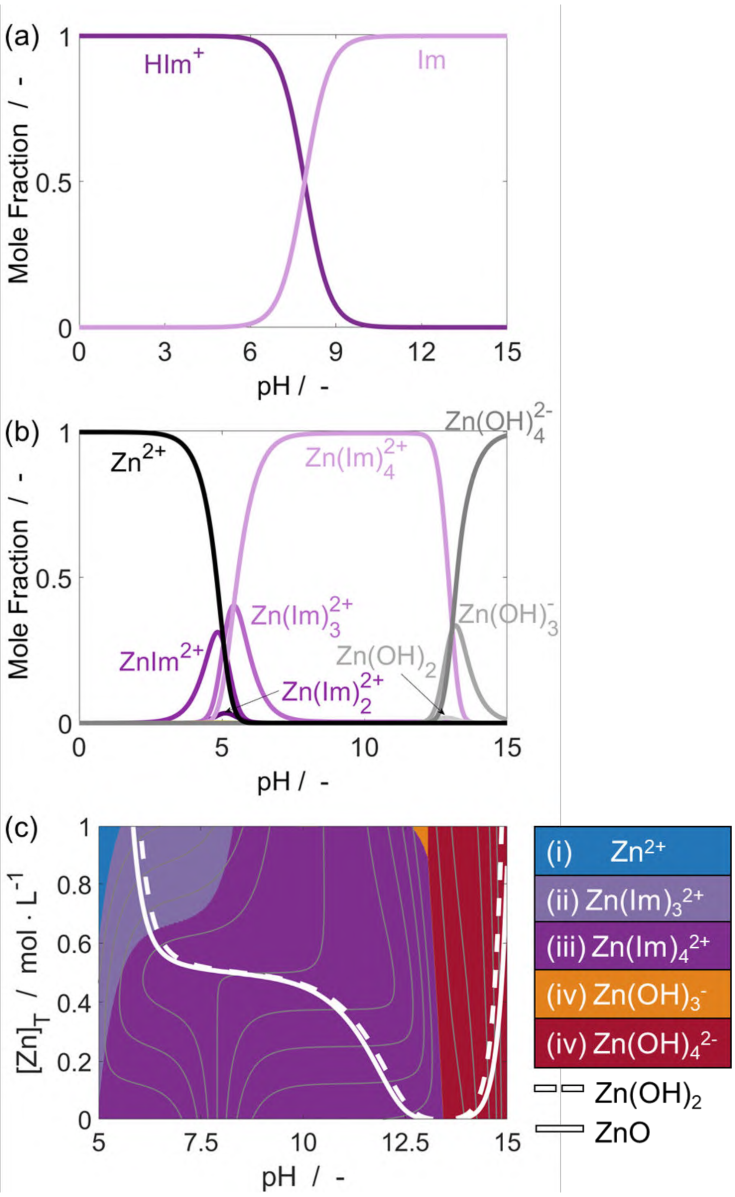


Figure S3. Speciation and solubility properties of imidizolium in aqueous zinc electrolytes. (a) Dissociation of 1M imidazolium, (b) speciation of 0.1M dissolved Zn in the solution, and (c) speciation and solubility landscape for $[\mathrm{Im}]_{\mathrm{T}} = 2\mathrm{M}$.

only donate a single proton, pH stability is susceptible to unfavorable concentration gradients that could occur during ZAB operation. Functional group modification (e.g. 4(2-Aminoethyl)imidazole) could address these challenges, but electrochemical oxidation of the electrolyte during charging could become a limiting factor.[62] We highlight imidazolium and its variants as materials of future interest, but do not analyze them here.

Table S9. Properties of the custom-made ZAB test cells.

| | **Exposed Area,** $cm^2$ | **Electrode Sep.,** cm | **Electrolyte Volume** |
|---|---|---|---|
| C1 | 1.327 $cm^2$ | 0.9 cm | 1.1 |
| C2 | 1.327 $cm^2$ | 2.8 cm | 4.4 |
| C3 | 1.327 $cm^2$ | 1.4 cm | 1.85 |

## S3. EXPERIMENTAL RESULTS

Properties of the custom-made cell designs used in this work are listed in Table S9.

### S3.1. Oxygen Electrocatalysis

To probe the electrochemical response at the common polycrystalline Pt (pc-Pt) electrode in the proposed electrolyte without and with oxygen, the reference measurements were first performed in the RRDE configuration (Figure S4). The underpotential adsorption/desorption of hydrogen (H-upd) is largely suppressed in both the base CV and the ORR (Figure S4a). This indicates the presence of adsorbed species at the Pt surface, as could be expected due to high concentration of citrate, glycine, and Zn(II) complexes in the solution, possibly resulting also in ZnO formation.[63] The current increase in the high potential regime indicates oxidation of organic components in the PtO region as expected for a typical Kolbe-type reaction for decarboxylation of carboxylic acids in both nitrogen and oxygen saturated electrolyte. The current peaks at ca. 1.45 V and 0.12 $mA\,cm^{-2}$. This corresponds to the small shoulder preceeding the exponential region observed in CNT and EMD+CNT catalyst

With the reduction of PtO, the ORR sets in and approaches a poorly resolved limiting current of ca. -0.15 $mA\,cm^{-2}$ in the potential range from ca. 0.5 to 0.07 V, which is much lower compared to typical mass transport limited ORR value of ca. -5.5 $mA\,cm^{-2}$ for Pt electrodes in diluted supporting electrolytes. This can be understood considering the above mentioned blocking of the electrode surface, as well as lower $O_2$ solubility[64] and a high kinematic viscosity in highly concentrated solutions. The hydrogen peroxide formation for the ORR at polycrystalline Pt disk electrode in the is not negligible, which can also indicates an impact of adsorbed species toward the $H_2O_2$ formation over a partly blocked Pt electrode.

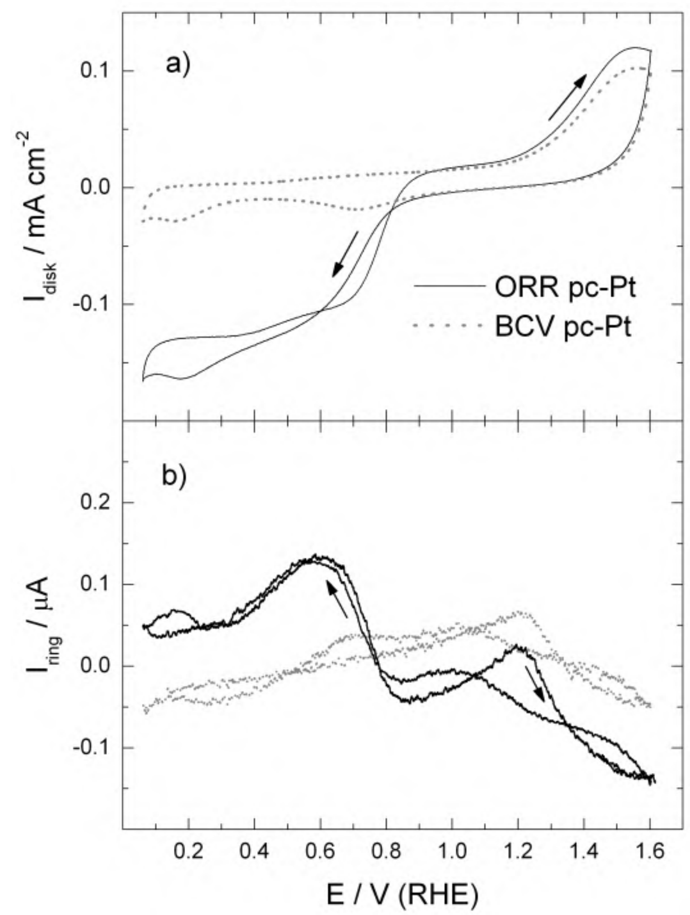


Figure S4. RRDE measurements at polycrystalline Pt electrode in an oxygen-saturated (black solid line) and oxygen-free (gray dotted line) aqueous $K_3$Cit−HGly−ZnO electrolyte. $\omega$ = 1600 rpm (ORR), scan rate = 10 mV s$^{-1}$, $U_{\mathrm{ring}}$ = 1.2 V. The disk current is shown in (a) and the ring current is shown in (b).

### S3.2. Full Cell Measurements

In addition to the constant current cycling experiments at 0.5 mA cm$^{-2}$ presented in the main text, results obtained at 1 mA cm$^{-2}$ are shown in Figure S5. This figure compares the cycling performance of ZAB C1 (containing 1.1 ml of electrolyte, black line) and C3 (containing 1.85 ml of electrolyte, blue line). The cell with the greater electrolyte volume achieved 59 cycles, while the cell with the smaller electrolyte volume achieved 39 cycles. The 51% gain in cycle lifetime correlates with the 68% increase in electrolyte volume.

The effects of charging protocol and electrolyte volume on cell cycling lifetime were investigated using full cell measurements. First, a constant voltage protocol, with the charging voltage was set to 2 V, was performed. The cell voltage profiles are shown in Figure S6. The results in Figure S6a were obtained at a discharging current of 0.5 mA cm$^{-2}$, and the results in Figure S6a were obtained at a discharging current of 1 mA cm$^{-2}$. The constant voltage results show a slight improvement of circa 11% in cycling life over constant current cycling. A summary of all the full cell cycling experiments is provided in Table S10.

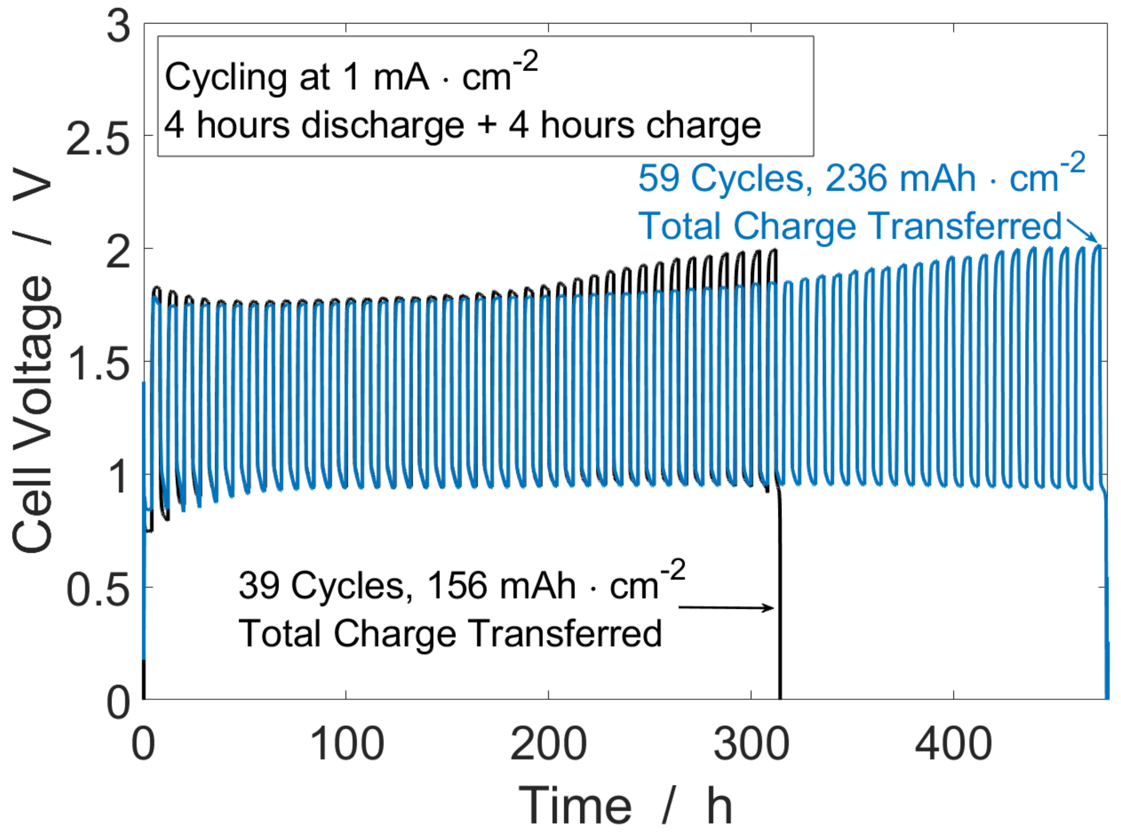


Figure S5. Cell voltage during cycling for a cell with (black) 1.1 ml electrolyte and (blue) 1.85 ml electrolyte.

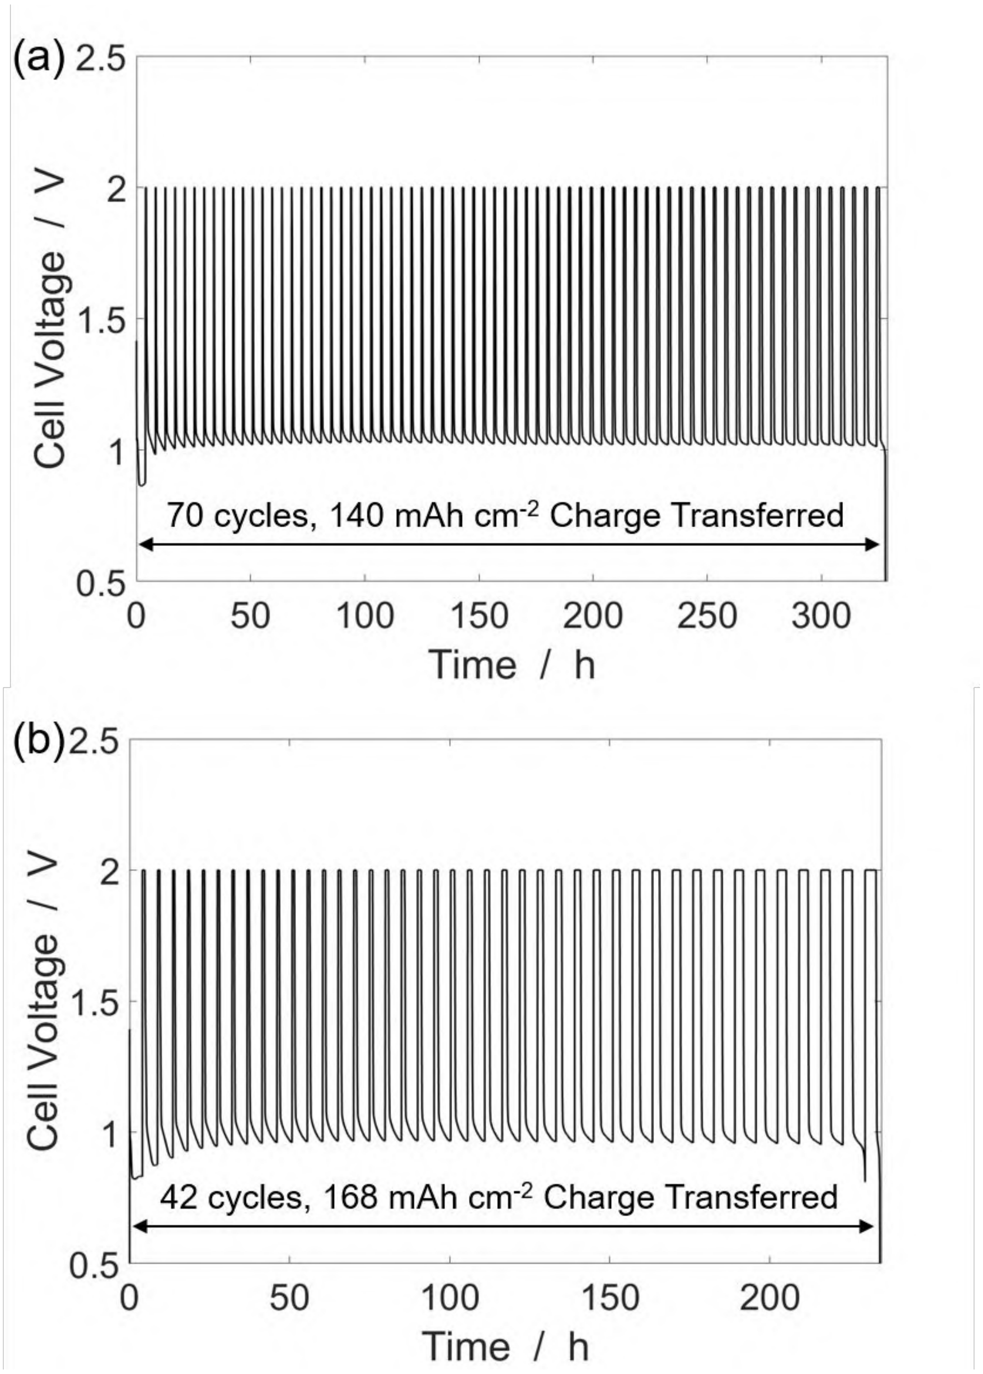


Figure S6. Comparison of cell voltages obtained with a constant voltage charging protocol ($U_{\text{charge}} = 2$ V) and constant current discharge at (a) 0.5 $\text{mA cm}^{-2}$ and (b) 1 $\text{mA cm}^{-2}$.

The total organic carbon content of the electrolyte was characterized under 3 conditions: (i) as prepared, (ii) after 400 hours of exposure to air, and (iii) after 416 hours of full cell cycling at 0.5 $\text{mA cm}^{-2}$. The results are summarized in Table S11.

The carbon content in the as prepared electrolyte is 100% organic, corresponding to the glcyine and citrate in the solution. After 400 hours of exposure to air, the total organic

Table S10. Summary of full cell cycling results achieved under various conditions.

| Cycling Protocol | Current / | Time / | Cycles / | Total Charge Transferred / | | |
|---|---|---|---|---|---|---|
| | $mA\,cm^{-2}$ | hour | - | $mA\,h\,cm^{-2}$ | $mA\,h\,g^{-1}{}_{Zn}$ | $mA\,h\,ml^{-1}{}_{Elyte}$ |
| 1.1 ml electrolyte | | | | | | |
| CC-CC | 0.5 | 4 | 63 | 126 | 706 | 139 |
| CC-CC | 0.5 | 8 | 26 | 104 | 582 | 115 |
| CC-CC | 1 | 4 | 39 | 156 | 874 | 173 |
| CC-CV | 0.5 | 4 | 70 | 140 | 784 | 155 |
| CC-CV | 1 | 4 | 42 | 168 | 941 | 186 |
| 1.85 ml electrolyte | | | | | | |
| CC-CC | 1 | 4 | 59 | 236 | 1321 | 174 |

Table S11. Total organic carbon content in the electrolyte under various conditions.

| **Condition** | **Total Organic Carbon** | **Other Carbon** |
|---|---|---|
| As Prepared | 100% | 0 % |
| 400 hours in air | 99% | 1% |
| 416 hours of cycling | 92% | 8% |

carbon content is 99%. The remaining 1% is attributable to ${CO_3}^{2-}$ formed as a result of exposure to $CO_2$ in the air. After 416 hours of cell cycling, the electrolyte is 92% organic carbon and 8% other carbon. This can be attributed to the combined effects of electrolyte oxidation and corrosion of the air electrode carbon support during cell charging. These results confirm that the electrolyte is stable in air, showing only minor degradation. The stability of both the electrolyte itself and the carbon gas diffusion electrode substrate during charging are topics for further research.

### S3.3. Zn Electrode Characterisation

The properties of a Zn electrode from a ZAB cell cycled at 0.5 mA cm$^{-2}$ for 7 cycles comprising 25 hours of discharging and 25 hours of charging (71.13 mAh $\cdot$ g$_{Zn}^{-1}$) were investigated with XRD, SEM, and EDS measurements. The powder XRD spectrum is shown in Figure S7. The XRD shows a mix of Zn metal (blue), ZnO (red), $Zn(OH)_2$ (yellow), and layered hydroxide (green).

A significant level of hkl-dependent peak intensity mismatch was observed in the fitting, particularly for the ZnO phase. This can be seen from a visual comparison of the diffraction patterns. This mismatch is indicative of highly anisotropic crystals, and was corrected for in the fitting via a spherical harmonics based intensity correction.

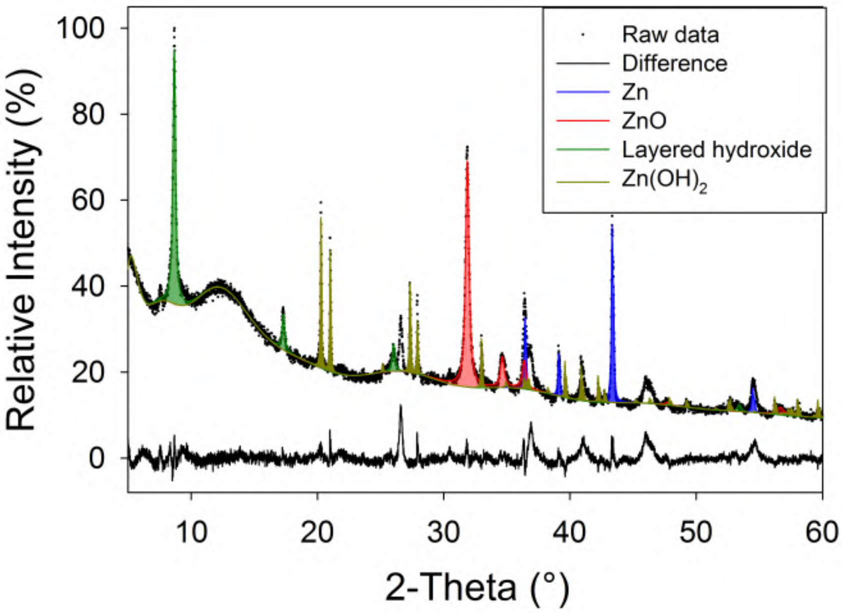


Figure S7. Powder XRD pattern for anode products formed after 7 discharge-charge cycles at a rate of 0.5 mA cm$^{-2}$ and for 25 hours discharging and 25 hours charging. Cycling was stopped midway through a charging step. Identified phases are fit and displayed in colour.

No phase in the available reference databases was found to match to the unknown phase with a strong low angle diffraction line, considering the system chemistry. A number of layered hydroxide phases are known to form when zinc is reacted under basic conditions though, the best known being $Zn_5(OH)_8Cl_2 \cdot H_2O$ (Simonkolleite),[65] $Zn_5(CO_3)_2(OH)_6$ (Hydrozincite) ADD CITATION GHOSE and $Zn_5(OH)_8(NO_3)_2 \cdot 2\,H_2O$ ADD CITATION STAEHLIN. These materials exhibit a similar diffraction pattern to this unknown phase, and as a good fit was achieved for the first 3 indexes of {00l} reflections, it is concluded that the phase is a layered hydroxide of some form. Such materials exhibit a layered structure

comprising metal hydroxide layers separated (or pillared) by a molecular species, with a c-axis unit cell length which is heavily sensitive to the intercalated species. A c-axis unit cell length (and thus interlayer spacing) in the range 10.28 Å to 10.31 Å was calculated. Though the nature of the intercalating species is not known here, it is noted that this value is similar to that reported for an ammonia-exchange sample of $Zn_5(OH)_8(NO_3)_2 \cdot 2\,H_2O$.[66]

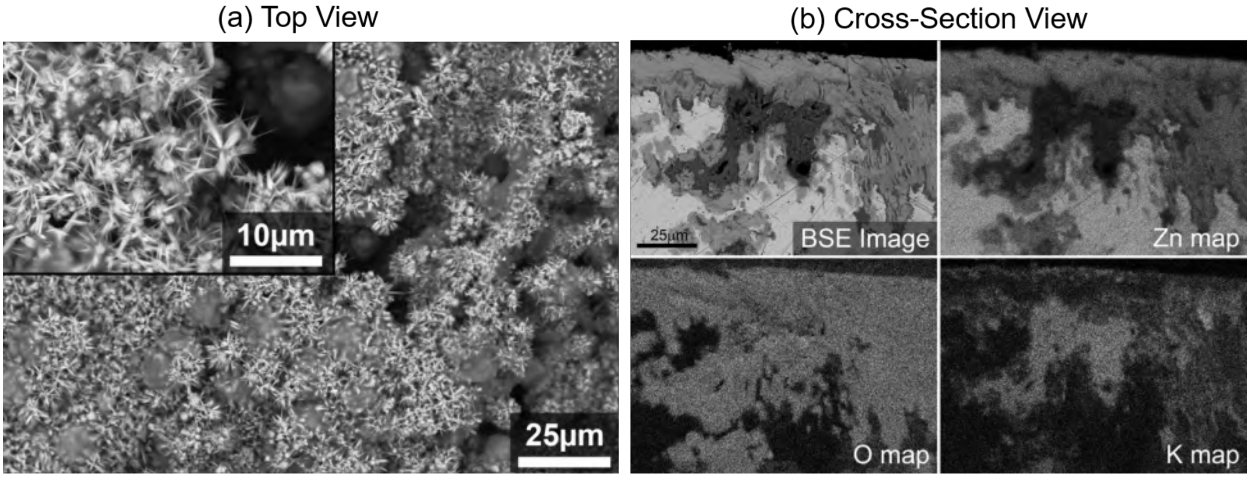


Figure S8. Backscattered electron image of a Zn electrode after 7 discharge-charge cycles at a rate of 0.5 $mA\,cm^{-2}$ and for 25 hours discharging and 25 hours charging. Cycling was stopped on a charging step. The figure shows (a) a top view with magnified inset of the same area, and (b) a cross section of the electrode with EDS elemental analysis. This sample corresponds to the XRD spectra shown in Figure S7.

Figure S8 shows (a) the top and (b) the cross-sectional backscattered electron images of the the Zn electrode corresponding to the XRD spectrum in Figure S7. The top view images of a cycled electrode show two crystal morphologies: a needle-like phase and a phase with smaller, more spherical morphology. ZnO is reported to grow in a needle like morphology .[67]

Potassium is also observed in all samples. No potassium-containing phase was identified in the XRD patterns, and none of the identified phases are known to incorporate potassium to any significant concentration. It is assumed that the potassium is present in an amorphous phase, formed from residual electrolyte which has dried after cell disassembly. As the composition of the K-containing component is unknown, and the K present everywhere, it was not possible to extract reliable quantitative compositional data via EDS to correlate microstructure to the phases observed by XRD.

Recent studies of zinc electrodes have called for establishing common benchmarks to facilitate cross-comparisons. To support this effort, in Table S12 we report some of the Zn electrode descriptors defined by Stock, et al.[68] for which we have data available. It should

be noted that the Zn electrode used in this work is a simple Zn foil.

Table S12. Descriptors for the common benchmarking of Zn anodes, according to the guidelines and mean values published by Stock, et al.[68]

| Descriptor | This Work | Lit. Mean[68] | Description |
|---|---|---|---|
| $m_{\mathrm{AM}}/m_{\mathrm{anode}}$ | 1 | $0.85 \pm 0.13$ | mass ratio of active material (AM) and anode mixture (AM and additives), - |
| $j_{\mathrm{dis}}$ | 1 | $13 \pm 11$ | discharging current density, $\mathrm{mA\,cm^{-2}}$ |
| $Q_{\mathrm{AM}}/V_{\mathrm{E}}$ | 176.4 | $227 \pm 242$ | ratio of capacity of AM and volume of electrolyte, $\mathrm{mA\,h\,ml^{-1}}$ |
| $N_{\mathrm{C}}$ | 63 | $483 \pm 624$ | number of cycles, - |
| $X_{\mathrm{AM}}$ | 1.37% | $44\% \pm 23\%$ | averaged utilization of AM, % |
| $q_{\mathrm{dis}}$ | 11.2 | $211 \pm 125$ | averaged discharge capacity per mass of anode mixture, $\mathrm{mA\,h\,g^{-1}}$ |
| $N_{\mathrm{C}} \cdot q_{\mathrm{dis}}$ | 706.8 | $322 \pm 561$ | product of averaged discharge capacity per mass of anode mixture and number of cycles, $\mathrm{mA\,h\,g^{-1}}$ |

[1] S. Clark, A. Latz, B. Horstmann. *ChemSusChem* **2017**, *10* 4735.

[2] S. Clark, A. R. Mainar, E. Iruin, L. C. Colmenares, J. R. Tolchard, A. Latz, B. Horstmann. *J. Mater. Chem. A* **2019**, *7* 11387.

[3] J. Stamm, A. Varzi, A. Latz, B. Horstmann. *J. Power Sources* **2017**, *360* 136.

[4] B. Horstmann, T. Danner, W. G. Bessler. *Energy Environ. Sci.* **2013**, *6* 1299.

[5] J. P. Neidhardt, D. N. Fronczek, T. Jahnke, T. Danner, B. Horstmann, W. G. Bessler. *J. Electrochem. Soc.* **2012**, *159* A1528.

[6] J. Limpo, A. Luis. *Hydrometallurgy* **1993**, *32* 247.

[7] J. Limpo, A. Luis, M. Cristina. *Hydrometallurgy* **1995**, *38* 235.

[8] J. Vazquez-Arenas, F. Sosa-Rodriguez, I. Lazaro, R. Cruz. *Electrochim. Acta* **2012**, *79* 109.

[9] M. Pourbaix. *Atlas of Electrochemical Equilibria in Aqueous Solutions.* National Association of Corrosion Engineers, Houston, Texas, 2nd edition, **1974**.

[10] R. Smith, A. Martell. *Critical Stability Constants*, volume 4. Springer, New York, NY, **1976**.

[11] A. Martell, R. Smith. *Other Organic Ligands.* Springer, New York, 1st edition, **1977**.

[12] X. G. Zhang. *Corrosion and Electrochemistry of Zinc.* Plenum Press, New York, NY, 1st edition, **1996**.

[13] J. Newman, K. E. Thmoas-Alyea. *Electrochemical Systems.* John Wiley & Sons, Hoboken, New Jersey, 3rd edition, **2004**.

[14] A. Latz, J. Zausch. *Electrochim. Acta* **2013**, *110* 358.

[15] S. Clark, A. Latz, B. Horstmann. *Batteries* **2018**, *4* 5.

[16] A. Zirino, S. Yamamoto. *Limnol. Oceanogr. Methods* **1972**, *17* 661.

[17] R. M. Smith, A. E. Martell. *Critical Stability Constants*, volume 5. Springer, New York, **1976**.

[18] H. L. Clever, M. E. Derrick, S. A. Johnson. *J. Phys. Chem. Ref. Data* **1992**, *21* 941.

[19] A. Moezzi, M. Cortie, A. M. McDonagh. *European Journal of Inorganic Chemistry* **2013**, *2013* 1326.

[20] S. Sobel, A. Haigney, T. Conception, M. Kim. *Chem. Speciation Bioavail.* **2008**, *20* 93.

[21] Z. Huajun, G. Zhenghai, Z. Jinhuan. *Hydrometallurgy* **2007**, *89* 369.

[22] A. Apelblat. *Citric Acid*, volume 1. Springer, **2015**.

[23] E. S. Hamborg, W. P. M. Van Swaaij, G. F. Versteeg. *J. Chem. Eng. Data* **2008**, *53* 1141.

[24] E. Iruin, A. R. Mainar, M. Enterría, N. Ortiz-Vitoriano, J. A. Blázquez, L. C. Colmenares, T. Rojo, S. Clark, B. Horstmann. *Electrochim. Acta* **2019**, *320* 134557.

[25] D. Eberle, B. Horstmann. *Electrochim. Acta* **2014**, *137* 714.

[26] T. Schmitt, T. Arlt, I. Manke, A. Latz, B. Horstmann. *J. Power Sources* **2019**, *432* 119.

[27] H. Pan, Y. Shao, P. Yan, Y. Cheng, K. S. Han, Z. Nie, C. Wang, J. Yang, X. Li, P. Bhattacharya, K. T. Mueller, J. Liu. *Nat. Energy* **2016**, *1* 16039.

[28] D. Kundu, B. D. Adams, V. Duffort, S. H. Vajargah, L. F. Nazar. *Nat. Energy* **2016**, *1* 16119.

[29] D. Kundu, S. Hosseini Vajargah, L. Wan, B. Adams, D. Prendergast, L. F. Nazar. *Energy Environ. Sci.* **2018**, *11* 881.

[30] F. Wan, L. Zhang, X. Dai, X. Wang, Z. Niu, J. Chen. *Nat. Commun.* **2018**, *9* 1656.

[31] B. Lee, H. R. Seo, H. R. Lee, C. S. Yoon, J. H. Kim, K. Y. Chung, B. W. Cho, S. H. Oh. *ChemSusChem* **2016**, *9* 2948.

[32] J. Jindra, J. Mrha, M. Musilová. *J. Appl. Electrochem.* **1973**, *3* 297.

[33] S. Huang, J. Zhu, J. Tian, Z. Niu. *Chem. Eur. J.* **2019**, chem.201902660.

[34] J. Garche, C. Dyer, P. Moseley, Z. Ogumi, D. Rand, B. Scrosati. *Encyclopedia of Electrochemical Power Sources*. Elsevier B.V., Amsterdam, **2009**.

[35] P. Leblanc, P. Blanchard, S. Senyarich. *J. Electrochem. Soc.* **1998**, *145* 844.

[36] M. G. Freire, C. M. S. S. Neves, I. M. Marrucho, J. A. P. Coutinho, A. M. Fernandes. *J. Phys. Chem. A* **2010**, *114* 3744.

[37] R. E. Mesmer, K. M. Palen, C. F. Baes. *Inorg. Chem.* **1973**, *12* 89.

[38] X. Liu, H. Zhang, D. Geiger, J. Han, A. Varzi, U. Kaiser, A. Moretti, S. Passerini. *Chem. Commun.* **2019**, *55* 2265.

[39] N. Zhang, F. Cheng, Y. Liu, Q. Zhao, K. Lei, C. Chen, X. Liu, J. Chen. *J. Am. Chem. Soc.* **2016**, *138* 12894.

[40] F. Wang, O. Borodin, T. Gao, X. Fan, W. Sun, F. Han, A. Faraone, J. A. Dura, K. Xu, C. Wang. *Nat. Mater.* **2018**, *17* 543.

[41] S. Amendola. *WO Patent* **2017**, WO 2017/142990 A1.

[42] M. S. Ghazvini, G. Pulletikurthi, T. Cui, C. Kuhl, F. Endres. *J. Electrochem. Soc.* **2018**, *165* D354.

[43] W. Lei, Y. P. Deng, G. Li, Z. P. Cano, X. Wang, D. Luo, Y. Liu, D. Wang, Z. Chen. *ACS Catal.* **2018**, *8* 2464.

[44] J. Zhang, G. Jiang, P. Xu, A. G. Kashkooli, M. Mousavi, A. Yu, Z. Chen. *Energy Environ. Sci.* **2018**, *11* 2010.

[45] Y. Li, M. Gong, Y. Liang, J. Feng, J.-E. Kim, H. Wang, G. Hong, B. Zhang, H. Dai. *Nat. Commun.* **2013**, *4* 1805.

[46] J. Lee, B. Hwang, M. S. Park, K. Kim. *Electrochim. Acta* **2016**, *199* 164.

[47] M. Schlesinger, M. Paunovic, editors. *Modern Electroplating*. John Wiley & Sons, Hoboken, New Jersey, 5 edition, **2011**.

[48] F. R. Mclarnon, E. J. Cairns. *J. Electrochem. Soc.* **1991**, *138* 645.

[49] S. Chen, J. Duan, P. Bian, Y. Tang, R. Zheng, S. Z. Qiao. *Adv. Energy Mater.* **2015**, *5* 1.

[50] Q. Liu, Y. Wang, L. Dai, J. Yao. *Adv. Mater.* **2016**, *28* 3000.

[51] Y. Huang, W. S. Ip, Y. Y. Lau, J. Sun, J. Zeng, N. S. S. Yeung, W. S. Ng, H. Li, Z. Pei, Q. Xue, Y. Wang, J. Yu, H. Hu, C. Zhi. *ACS Nano* **2017**, *11* 8953.

[52] X. Guo, T. Zheng, G. Ji, N. Hu, C. Xu, Y. Zhang. *J. Mater. Chem. A* **2018**, *6* 10243.

[53] Z. Xie, Q. Su, A. Shi, B. Yang, B. Liu, J. Chen, X. Zhou, D. Cai, L. Yang. *Journal of Energy Chemistry* **2016**, *25* 495.

[54] S. Amendola, M. Binder, P. J. Black, S. Sharp-Goldman, L. Johnson, M. Kunz, M. Oster, T. Chciuk, R. Johnson. *US Patent* **2012**, US 2012/0021303 A1.

[55] B. K. Thomas, D. J. Fray. *J. Appl. Electrochem.* **1981**, *11* 677.

[56] J. L. Ortiz-Aparicio, Y. Meas, G. Trejo, R. Ortega, T. W. Chapman, E. Chainet, P. Ozil. *Electrochim. Acta* **2007**, *52* 4742.

[57] J. C. Ballesteros, E. Chaînet, P. Ozil, G. Trejo, Y. Meas. *Electrochim. Acta* **2011**, *56* 5443.

[58] D. G. Marangoni, R. S. Smith, S. G. Roscoe. *Can. J. Chem.* **1989**, *67* 921.

[59] H. V. M. Hamelers, A. Ter Heijne, T. H. J. A. Sleutels, A. W. Jeremiasse, D. P. B. T. B. Strik, C. J. N. Buisman. *Appl. Microbiol. Biotechnol.* **2010**, *85* 1673.

[60] Z. Liu, P. Bertram, F. Endres. *J. Solid State Electrochem.* **2017**, *21* 2021.

[61] T. L. Amyes, S. T. Diver, J. P. Richard, F. M. Rivas, K. Toth. *J. Am. Chem. Soc.* **2004**, *126* 4366.

[62] B. V. Sarada, T. N. Rao, D. A. Tryk, A. Fujishima. *Anal. Chem.* **2000**, *72* 1632.

[63] M. Stumpp, T. H. Nguyen, C. Lupo, D. Schlettwein. *Electrochim. Acta* **2015**, *169* 367.

[64] M. Geng, Z. Duan. *Geochim. Cosmochim. Acta* **2010**, *74* 5631.

[65] C. Hawthorne. *Can. Mineral.* **2002**, *40* 939.

[66] G. G. C. Arízaga. *J. Solid State Chem.* **2012**, *185* 150.

[67] A. Kolodziejczak-Radzimska, T. Jesionowski. *Materials* **2014**, *7* 2833.

[68] D. Stock, S. Dongmo, J. Janek, D. Schröder. *ACS Energy Lett.* **2019**, *4* 1287 .
